# Supplementary material for: An Attention-based Representation Distillation Baseline for Multi-Label Continual Learning
Source: arXiv:2407.14249 source file (2024-07-19)
Supplement: Supplementary file 1 [file appendix.tex]

\subsection{Training details}
We use the same network architecture, a pretrained ViT-B/16, for all benchmarked models. For ER, ER-ACE, DER++-ACE, L2P and SCAD we use SGD as the optimizer, with a learning rate of $0.03$. Although the authors of L2P use Adam as the optimizer, with SGD we achieved better results. For CP, we use Adam with a learning rate of $0.001$, as described in its original paper~\citep{smith2022coda}. For all models except CP, we also apply gradient norm clipping with a maximum norm value of $1.0$, as we noticed that this improves the model's performance. For the sake of fairness, we train all methods for the same amount of epochs and keeping the same batch size.

\subsection{Hyperparameters}
We report in Table \ref{tab:sup_hyp_iirc} and in Table \ref{tab:sup_hyp_webvision} the hyperparameters used for the IIRC-CIFAR100 and WebVision benchmarks respectively.

 \begin{table}[H]
    \centering
    \caption{Hyperparameters used for the IIRC-CIFAR100 benchmark.}
    % \resizebox{.42\paperheight}{!}{%
    \begin{tabular}{ccl}%@{\hskip 0.5cm}
    \noalign{\smallskip}
    \hline
    \noalign{\smallskip}

\multicolumn{3}{c}{\textbf{IIRC CIFAR100 - Class-IL}}\\\noalign{\smallskip}
    \hline
    \noalign{\smallskip}
\textit{shared} & &  $\text{Eps}: 5$ $\text{bs}: 16$ \\
\noalign{\smallskip}
\hline
\noalign{\smallskip}
\textbf{Method} & \textbf{Buffer size} & \textbf{Other parameters} \\
\noalign{\smallskip}
\hline
\noalign{\smallskip}
JOINT & - &$\text{lr}:0.03$ \\
SGD & - &$\text{lr}:0.03$ \\
L2P \cite{wang2022learning} & - &$\text{lr}:0.03$ $\;\text{pool\_size}: 10$ \\
CP \cite{smith2022coda} & - &$\text{lr}:0.001$ $\;\text{pool\_size}: 100$\\
ER \cite{ratcliff1990connectionist,robins1995catastrophic} & $500$ &$\text{lr}:0.03$ \\
  & $2000$ &$\text{lr}:0.03$ \\
ER-ACE \cite{caccia2022new} & $500$ &$\text{lr}:0.03$ \\
  & $2000$ &$\text{lr}:0.03$ \\
\dpp \cite{buzzega2020dark} & $500$ &$\text{lr}:0.03$ $\alpha:0.3$ $\beta:0.8$ \\
  & $2000$ &$\text{lr}:0.03$ $\alpha:0.3$ $\beta:0.8$ \\
\methnam & $500$ &$\text{lr}:0.03$ $\alpha:0.3$ $\beta:0.8$ $\lambda_\text{FP}:1.0$ $\lambda_{\text{FP\_rep}}:0.1$ $\mathcal{L}:\{1,4,7,10\}$ \\
  & $2000$ &$\text{lr}:0.03$ $\alpha:0.3$ $\beta:0.8$ $\lambda_\text{FP}:1.0$ $\lambda_{\text{FP\_rep}}:0.1$ $\mathcal{L}:\{1,4,7,10\}$ \\
\noalign{\smallskip}
    \hline
    \noalign{\smallskip}
    \end{tabular}
    
    % }
\label{tab:sup_hyp_iirc}
\end{table}

\clearpage

 \begin{table}[H]
    \centering
    \caption{Hyperparameters used for the WebVision benchmark.}
    % \resizebox{.42\paperheight}{!}{%
    
    \begin{tabular}{ccl}%@{\hskip 0.5cm}
\noalign{\smallskip}
    \hline
    \noalign{\smallskip}
    
\multicolumn{3}{c}{\textbf{WebVision - Class-IL}}\\\noalign{\smallskip}
    \hline
    \noalign{\smallskip}
\textit{shared} &&  $\text{Eps}: 1$ $\text{bs}: 16$ \\
\noalign{\smallskip}
\hline
\noalign{\smallskip}
\textbf{Method} & \textbf{Buffer size} & \textbf{Other parameters} \\
\noalign{\smallskip}
\hline
\noalign{\smallskip}
JOINT & - &$\text{lr}:0.03$ \\
SGD & - &$\text{lr}:0.03$ \\
L2P \cite{wang2022learning} & - &$\text{lr}:0.03$ $\;\text{pool\_size}: 10$ \\
CP \cite{smith2022coda} & - &$\text{lr}:0.001$ $\;\text{pool\_size}: 100$ \\
ER \cite{ratcliff1990connectionist,robins1995catastrophic} & $2000$ &$\text{lr}:0.03$ \\
  & $5000$ &$\text{lr}:0.03$ \\
ER-ACE \cite{caccia2022new} & $2000$ &$\text{lr}:0.03$ \\
  & $5000$ &$\text{lr}:0.03$ \\
\dpp \cite{buzzega2020dark} & $2000$ &$\text{lr}:0.03$ $\alpha:0.3$ $\beta:0.9$ \\
  & $5000$ &$\text{lr}:0.03$ $\alpha:0.3$ $\beta:0.9$ \\
\methnam & $2000$ &$\text{lr}:0.03$ $\alpha:0.3$ $\beta:0.9$ $\lambda_\text{FP}:1.0$ $\lambda_{\text{FP\_rep}}:0.1$ $\mathcal{L}:\{1,4,7,10\}$ \\
  & $5000$ &$\text{lr}:0.03$ $\alpha:0.3$ $\beta:0.9$ $\lambda_\text{FP}:1.0$ $\lambda_{\text{FP\_rep}}:0.1$ $\mathcal{L}:\{1,4,7,10\}$ \\
\noalign{\smallskip}
    \hline
    \noalign{\smallskip}
    \end{tabular}
    
    % }
    \label{tab:sup_hyp_webvision}
\end{table}
%     \label{tab:hyperpc10}
% \end{table}

\subsection{SCAD algorithm}
The pseudocode in Algorithm \ref{alg:scad} outlines the sequence of operations of our method. 
%$F_\mathcal{T}$ and $F_\mathcal{S}$ are the intermediate representations of teacher and student respectively. $N$ is the number of tokens of the Vision Transformer. $W_1$, $W_2$ are two vectors of learnable weights and $b1$, $b2$ are two learnable biases. $\mathcal{L}$ is the set of layers where we perform the distillation.
\begin{algorithm}[H]
\caption{SCAD algorithm}\label{alg:scad}
\setstretch{1.2}
\begin{algorithmic}
\Require Intermediate representations $F_\mathcal{T}$, $F_\mathcal{S}$, number of tokens $N$, weights $W_1$, $W_2$,\\\hspace{3.3em}biases $b_1$, $b_2$, adapter layers $\mathcal{L}$
\State $loss_\text{\,FP} \gets 0$
\For{$l\:\textbf{in}\:\mathcal{L}$}
\State $norm\_F_\mathcal{T} \gets F_\mathcal{T}^l / ||F_\mathcal{T}^l||_2^2$
\State $norm\_F_\mathcal{S} \gets F_\mathcal{S}^l / ||F_\mathcal{S}^l||_2^2$
\State $\mathcal{R}_\mathcal{T} \gets norm\_F_\mathcal{T} \cdot norm\_F_\mathcal{T}^T $
\State $\mathcal{R}_\mathcal{S} \gets norm\_F_\mathcal{S} \cdot norm\_F_\mathcal{S}^T $
\State $attn\_vec_\mathcal{T} \gets \mathcal{R}_\mathcal{T}\left[ 0,1:N+1 \right]$
\State $attn\_vec_\mathcal{S} \gets \mathcal{R}_\mathcal{S}\left[ 0,1:N+1 \right]$

\State $bin\_vec \gets gumbel(stack(attn\_vec_\mathcal{T} \odot W_1 + b_1, attn\_vec_\mathcal{T} \odot W_2 + b_2))$

\State $dist \gets bin\_vec \odot (attn\_vec_\mathcal{T} - attn\_vec_\mathcal{S})^2$
\State $loss_\text{\,FP} \gets loss_\text{\,FP} + mean(dist)$
\EndFor
\State $\mathcal{L}_\text{FP} \gets \lambda_\text{FP} \cdot \frac{1}{|L|} loss_\text{\,FP}$

\end{algorithmic}
\end{algorithm}
